# Supplementary material for: Prandtl-Tietjens intermittency in transitional pipe flows
Source: arXiv:2110.14983 ancillary file (2022-01-13)
Supplement: Supplementary file 1 [file SupplementaryMaterial.pdf]

# Prandtl-Tietjens intermittency in transitional pipe flows: Supplementary Material

## CONTENTS


I. Derivation of Eq. 1 — 1

II. Improving time resolution and determining $l$, $u_F$, and $u_B$ experimentally — 2

III. Using the Barkley model [1] for $l$ — 4

IV. Rotta's pressure-driven experiments [2] — 6

V. Estimate of external resistance $R$ from Barkley et al. [1] — 6

References — 6


## I. DERIVATION OF EQ. 1

Here we provide a more detailed derivation of Eq. 1 in the main text used to determine the Reynolds number $Re = UD/\nu$ from a constant pressure drop, where $U$ is the cross-sectional average velocity, $D$ is the pipe diameter, and $\nu$ is the kinematic viscosity. We start with an expression for the total pressure drop $\Delta P_{\text{tot}}$ in the pipe system, which is set by the reservoir height minus the outlet height, $\Delta h$, and which is assumed constant in each experiment. This is split between the pressure drop in the actual pipe, $\Delta P_{\text{pipe}}$, and the pressure drop in the hoses, entrance section, flowmeter section, etc., external to the experimental pipe section but in the pipe system, $\Delta P_{\text{ext}}$. (Importantly, we also include the section of the pipe of length $\simeq 400D$ before the perturbation as part of the external resistance, since it includes developing flow that will not conform to the laminar friction law.) We write this split as

$$\Delta P_{\text{tot}} = \Delta P_{\text{pipe}} + \Delta P_{\text{ext}}. \tag{S1}$$

Next we determine the dependence of $\Delta P_{\text{pipe}}$ on $Re$, which will also enable us to empirically determine the dependence of $\Delta P_{\text{ext}}$ on $Re$. If the flow is laminar, then we know that the normalized pressure drop, the friction factor $f$, goes as $f = 64/Re$, the Hagen-Poiseuille law, where $f$ is defined as

$$f = \frac{D\Delta P_{\text{pipe}}/L}{\frac{1}{2}\rho U^2}, \tag{S2}$$

where $L$ is the length of the pipe and $\rho$ is the density of the fluid. For fully-developed laminar flow, we have the Hagen-Poiseuille law $f = 64/Re$, so that we can write the pressure drop for laminar flow as:

$$\Delta P_{\text{pipe, laminar}} = \frac{32\rho\nu^2}{D^3} L Re. \tag{S3}$$

If instead the flow is fully turbulent, then we have the Blasius law: $f = 0.3164 Re^{-1/4}$, which gives

$$\Delta P_{\text{pipe, turbulent}} = \frac{0.3164\rho\nu^2}{2D^3} L Re^{7/4}. \tag{S4}$$

If the flow is in transition, where it is a mixture of laminar and turbulent flow (in the form of slugs), then $\Delta P_{\text{pipe}}$ will be a combination of Eq. S3 and Eq. S4, and the total length of the pipe $L$ in each will need to be replaced by the portion of the pipe filled by laminar flow and turbulent flow respectively. We will assume the turbulent pressure gradient relationship with $Re$ is the same for slugs, as has been shown in Ref. [3], and neglect any contribution from the interfaces. Since even short sections of laminar or slug flow were found to follow these friction laws [3], we also do not consider any finite-size effects from flow development. Calling $l$ the length of the pipe filled by the turbulent slug, the portion of the pipe that remains laminar is $L - l$. Eq. S1 then becomes

$$\Delta P_{\text{tot}} = \Delta P_{\text{pipe, laminar}} + \Delta P_{\text{pipe, turbulent}} + \Delta P_{\text{ext}} = \frac{32\rho\nu^2}{D^3}(L-l)Re + \frac{0.3164\rho\nu^2}{2D^3} l Re^{7/4} + \Delta P_{\text{ext}}. \tag{S5}$$

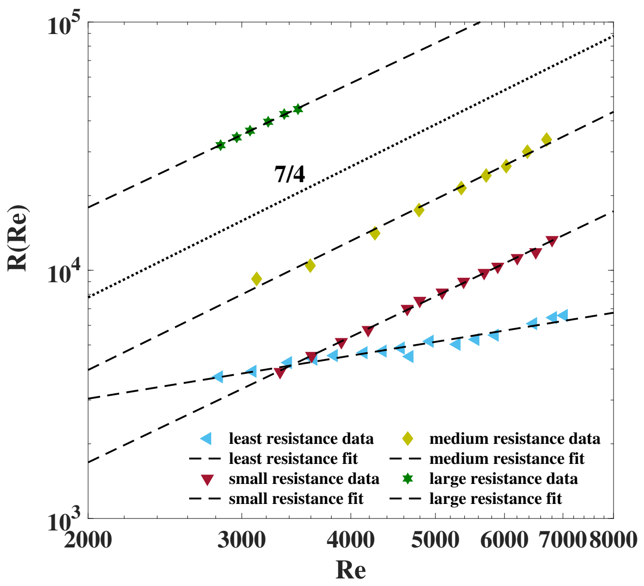


FIG. S1. Log-log plot of the non-dimensional external resistance, $R$, vs. $Re$. The variation with $Re$ is a power law for all cases with an exponent close to 7/4 when an external resistance is used. The best fits are $R = 0.0047687Re^{1.6806}$ ("small resistance"), $R = 0.00078503Re^{1.728}$ ("medium resistance"), and $R = 0.0578Re^{1.6634}$ ("large resistance").

Dividing both sides by $32\rho\nu^2 L/D^3$, yields a non-dimensional relation:

$$\frac{D^3 \Delta P_{\rm tot}}{32\rho\nu^2 L} = {\rm const.} = \left(1 - \frac{l}{L}\right) Re + B\frac{l}{L} Re^{7/4} + R, \tag{S6}$$

where $B = 0.3164/64$, a constant, and $R = \frac{D^3 \Delta P_{\rm ext}}{32\rho\nu^2 L}$ is the non-dimensional external resistance. Next we empirically determine $R$ as a function of $Re$ by conducting a series of experiments for which the pipe is fully laminar ($l = 0$) and adjust the height of the reservoir to change $\Delta P_{tot} = \rho g \Delta h$, where $g$ is the gravitational acceleration and $\Delta h$ is the difference in height between the reservoir and exit. Setting $l = 0$ in Eq. S6 yields:

$$R = \frac{D^3 \Delta P_{\rm tot}}{32\rho\nu^2 L} - Re. \tag{S7}$$

The external resistance includes sections with non-uniform and changing cross-section so that it is not obvious that $R$ should be determined by either the Hagen-Poiseuille or Blasius friction factor laws. However, to explore the effect of the external resistance we vary it by adding several external "resistors" (as done, for example, by Ref. [4]). These consist of short, straight pipes with a smaller diameter than the experimental pipe section so that $Re$ inside them is high and the flow inside is expected to be always turbulent. These are placed at the end of the pipe system. The resistor pipe length $L_R$ and diameter $D_R$ for the "small resistance" are $L_R = 70$ cm and $D_R = 0.68$ cm, for the "medium resistance" are $L_R = 67$ cm and $D_R = 0.58$ cm, and for the "large resistance" are $L_R = 100$ cm and $D_R = 0.36$ cm. If the flow inside these is turbulent, we would expect the external resistance to scale as $Re^{7/4}$, as in Eq. S4, which the data in Fig. S1 indeed do show. However, we reiterate that the external resistance $R$ is not only due to these resistors, as substantiated by the fact that even without a resistor the "least resistance" $R$ is non-negligible.

## II. IMPROVING TIME RESOLUTION AND DETERMINING $l$, $u_F$, AND $u_B$ EXPERIMENTALLY

The response time of the magnetic flowmeter was at times insufficient to fully capture changes in $Re$, so we also use a Laser Doppler Velocimeter (LDV) to measure the velocity and calibrate this with the flowmeter to obtain a better temporal resolution. Since the LDV measurement position was upstream of the perturbations and sufficiently downstream of the entrance ($\simeq 400D$), the flow there is always fully-developed laminar flow. As an example time series of $Re(t)$ in Fig. S2 shows, the LDV is better able to capture the minimum in the $Re(t)$ curve, corresponding to

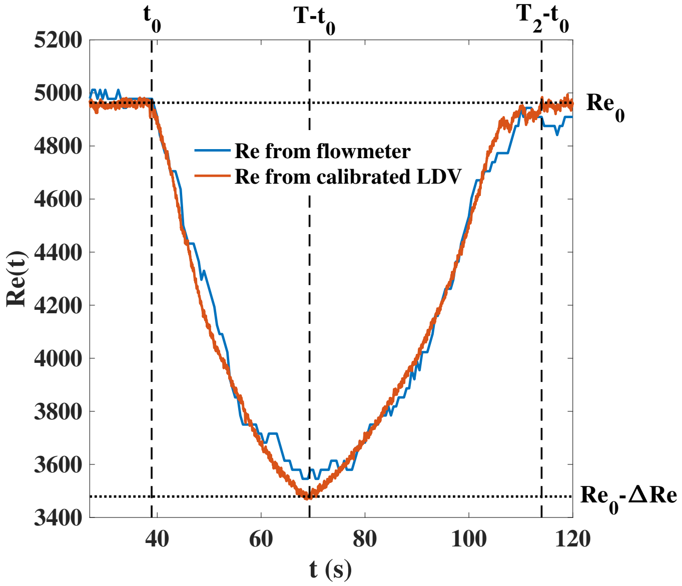


FIG. S2. Plot of $Re(t)$ vs. $t$ from one of the experiments used to determine $\Delta Re$ vs. $Re_0$ as in the main text. A measurement of the velocity upstream with an LDV is used to determine $Re(t)$ with better temporal resolution. Before the is perturbed at time $t_0$, the initial Reynolds number is $Re_0$. After $t_0$ a slug is generated which grows and moves downstream. Thus $Re(t)$ decreases until the slug front reaches the end of the pipe, which we identify as the minimum value $Re(t) = Re_0 - \Delta Re$, at a time $T - t_0$. Since the slug back continues to move toward the exit of the pipe, $Re(t)$ increases thereafter until the slug entirely exits the pipe at a time $T_2 - t_0$ which we identify as the point $Re(t) = Re_0$. From $T$ and $T_2$ we obtain estimates of $u_F$, $u_B$ and thus $l/L$, and from this plot we also obtain $Re_0$ and $\Delta Re$.

when the slug leaves the pipe, which enables a better estimate of the slug speed and the magnitude of the departure from the inital $Re_0$.

For our initial test of the model, Eqs. 1, 2 in the main text, we made our own estimates of $u_F$, $u_B$ and $l$. Referring to Fig. S2, we estimate the speeds and thus $l/L$ by identifying in the time series of $Re(t)$ the time when the flow was perturbed, $t_0$, the time when the slug front reaches the end of the pipe, $T - t_0$, and the time when the slug finally exits the pipe, $T_2 - t_0$, at which point the flow returns to its initial value $Re_0$. (The perturbation time $t_0$ is also known independently.) $T - t_0$ is identified with the minimum of $Re(t) = Re_0 - \Delta Re$, since before this time the slug is growing and so $Re(t)$ is decreasing, and after this point the slug will no longer grow since its front has reached the exit and thus $Re(t)$ will increase. $T_2 - t_0$ is identified with the point when $Re(t) = Re_0$, since this indicates that the back of the slug has reached the end of the pipe and the slug is now gone. From $T$ and $T_2$ we obtain the following estimates

$$u_F = \frac{L}{T}, \quad u_B = \frac{L}{T_2}. \tag{S1}$$

As argued in the main text, $T$ corresponds to the minimum in $Re(t)$ and thus the maximum in $l/L$ vis-à-vis Eq. S6. Thus $L = u_F T$ and $L - l = u_B T$ results in

$$\frac{l}{L} = \frac{u_F - u_B}{u_F} = 1 - \frac{T}{T_2}. \tag{S2}$$

As Fig. 2 in the main text shows, this results in predictions of $\Delta Re$ vs. $Re_0$ using Eq. 2 in the main text that are in excellent accord with the experimental results.

The estimates of $u_B$ and $u_F$ are not in agreement with previously (empirically) determined relations of $u_B/U$ and $u_B/U$ vs. $Re$ [1, 5]. The reason for this is that in those experiments and simulations the $Re$ was kept as constant as possible, whereas here we deliberately allowed $Re(t)$ to vary. If we use the relations of $u_B/U$ and $u_F/U$ vs. $Re$ from the literature to determine $l/L$ we are not able to accurately predict $\Delta Re$ vs. $Re_0$ for the smaller resistances (which have a larger deviation $\Delta Re$), as can be seen in Fig. S3. However, the predictions match well for the larger resistances, and the prediction of $\Delta Re$ using our model are in close agreement with the fluctuations in $Re$ quoted in Ref. [1] (see also Sec. III). Moreover we can also estimate the corresponding $\Delta Re$ in Rotta's experiments, which are also relatively small, in agreement with his observations.

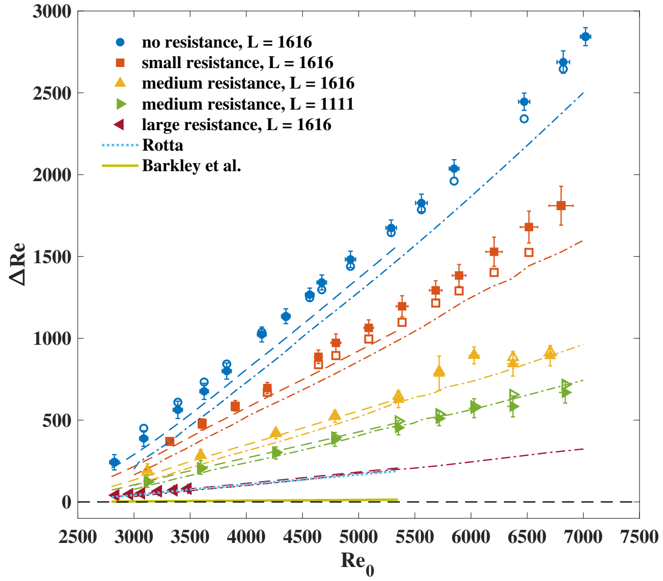


FIG. S3. Plot of deviation in $Re$, $\Delta Re$, vs. the initial laminar $Re_0$ for several different $R$. (This supplementary plot is similar to the plot in the main text, but with added predictions and estimates.) Increasing $R$ or decreasing $L$ reduces $\Delta Re$. The predicted $\Delta Re$, indicated by open symbols, is in excellent accord with the experimental data and in many cases indistinguishable from it. The dashed (−−) and dash-dot (−·−·) lines are the predictions of Eq. 2 in the main text using the $l/L$ found empirically by Ref. [1] and Ref. [5] respectively. We also include predictions of $\Delta Re$ for the experiments of Barkley et al. [1] (—) and Rotta [2] (· · ·) using the external resistance $R(Re)$ estimated below (see Secs. III, IV). For the estimates of Barkley et al. [1] (—) we also used the $u_F$ and $u_B$ they empirically determined to estimate $l/L$.

## III. USING THE BARKLEY MODEL [1] FOR $l$

The model used to determine the growth of $l$ was developed to investigate the dependence of slug front and back speeds on $Re$ [1]:

$$\frac{\partial q}{\partial t} + (u - \xi)\frac{\partial q}{\partial x} = f(q,u) + D\frac{\partial^2 q}{\partial x^2}, \tag{S3a}$$

$$\frac{\partial u}{\partial t} + u\frac{\partial u}{\partial x} = \epsilon g(q,u), \tag{S3b}$$

$$f(q,u) = q(r + u - 2 - (r + 0.1)(q-1)^2), \tag{S3c}$$

$$g(q,u) = 2 - u + 2q(1-u). \tag{S3d}$$

$q$ and $u$ represent the local turbulence intensity and local centerline speed of the pipe, respectively, and $r$, $\xi$, $D$ and $\epsilon$ are parameters that control the physics. More information can be found in the original publication [1], and we simply adopt the parameter values that they found give the best agreement with experiments: $D = 0.13$, $\xi = 0.79$, $\epsilon = 0.2$, and $r$ becomes the control parameter in a similar way to $Re$ for the experiments. Although there are strong links between parameters in the model and experimental parameters, they can not be rigorously established. Instead, if we make the assumption that the essential physics of the model and the experiments are the same, then we only need to determine an empirical relation between the front speeds and the inertial parameter $r$ and $Re$. This was already done by Ref. [1], who were able to fit their model interface speeds ($c$) to the experimental ones ($C$) by making the following transformations:

$$r = \frac{Re - Re_0}{Re_1 - Re_0}, \quad Re_0 = 1920, \quad Re_1 = 2250, \tag{S4a}$$

$$c = \frac{C - C_0}{2(C_1 - C_0)} + c_0, \quad C_0 = 1.06, \quad C_1 = 0.92, \tag{S4b}$$

where $c_0 = 2 - \xi = 1.21$, the capital $C$ refers to either the front ($u_F/U$) or back ($u_B/U$) speed normalized by the mean speed $U$, and a lowercase $c$ refers to the interface speeds in the model. These transformations are not arbitrary, but are determined by, for example, the speed and $Re$ at which the front and back interface speeds begin to diverge

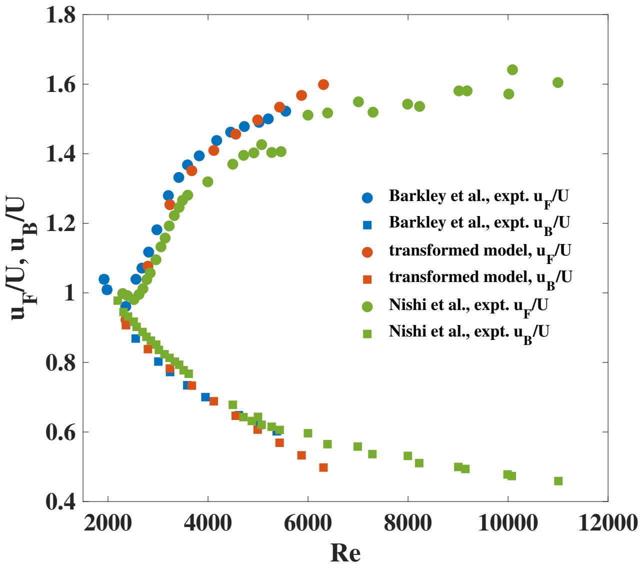


FIG. S4. Non-dimensional front and back speeds for slugs (and puffs). The data from the literature were extracted from article graphics using WebPlotDigitizer 4.2 (http://arohatgi.info/WebPlotDigitizer/). The front and back speeds using our new transformation (Eq. S5) are in excellent accord with previous experimental results.

from each other [1]. An important point for us is that this transformation is performed *after* the simulations are finished. The speeds, after being transformed, give the rate of change of the fraction of the flow that is turbulent $\frac{dl/L}{dt}$, but $l/L$ itself will be different. This is easily appreciated by noticing that for large values of $r$, the back speed of the turbulent region becomes negative. For example, at $r \simeq 9.33$ ($Re = \simeq 5000$), the experimental back speed is $C = u_B/U \simeq 0.624$, yielding $c \simeq -0.347$ with the parameters given above. This is not physically possible in the experiments, and we could find no simple transformation of the simulation domain to bring $l/L$ into correspondence with the experiments. Instead, through trial and error we determined that the following transformation of the original model equations bring them into accord with the experiments, without the need for a subsequent transformation:

$$r = \frac{Re - Re_0}{\gamma(Re_1 - Re_0)} \tag{S5a}$$

$$\frac{\partial q}{\partial t} + \alpha[(u-\xi)+\beta]\frac{\partial q}{\partial x} = f(q,u) + \alpha^2 D\frac{\partial^2 q}{\partial x^2}, \tag{S5b}$$

$$\frac{\partial u}{\partial t} + (\alpha u + \beta)\frac{\partial u}{\partial x} = \epsilon g(q,u), \tag{S5c}$$

$$f(q,u) = q(r + u - 2 - (r+0.1)(q-1)^2), \tag{S5d}$$

$$g(q,u) = 2 - u + 2q(1-u), \tag{S5e}$$

where $\alpha$, $\beta$, and $\gamma$ are new parameters given by

$$\alpha = 2(C_0 - C_1), \quad \beta = C_0 - 2\alpha(2-\xi), \quad \gamma = 1.3. \tag{S6}$$

The nonlinear terms in the original model, Eqs. S5d, S5e, remain unchanged. The transformation amounts to a new mapping of $Re$ to $r$, Eq. S5a, and modifications to the convection speed and diffusion, Eqs. S5b, S5c. After this transformation, we estimated the front and back speeds once again and found good agreement with the literature data [1, 5] (see Fig. S4). Since these empirical data are for (approximately) constant $Re$, using a model to simulate slug growth for a varying $Re(t)$ implicitly assumes a kind of quasi-static approximation, where the slug front and back speeds follow the constant $Re$ curves in Fig. S4 during the short integration times, with speeds that correspond to the instantaneous $Re(t)$.

## IV. ROTTA'S PRESSURE-DRIVEN EXPERIMENTS [2]

Rotta's experiments using water were very similar to our own, with a reservoir raised above the exit of the pipe to provide a constant pressure drop [2]. He apparently pioneered the idea of introducing a large flow resistance in order to try and maintain a constant (on average) $Re$ during the transition. We can estimate the external resistance $R$ of his resistor (effected by the valve used to control the flow rate). To estimate $R(Re)$, we use Eq. S7, where $\Delta P_{\rm tot} = \rho g h$, and we take a case where the flow is fully laminar. We also assume that like our external resistances, $R(Re) \propto Re^{7/4}$. Based on the information provided in the paper and methods section:

- $\Delta h = 700$ cm.
- $D = 0.27$ cm. (This more precise value of the diameter is given in Fig. 17 of Rotta's paper.)
- The pipe length is 150 cm, and the perturbation is assumed to be effected at the entrance, so that $L = 150$ cm $\simeq 556D$.
- The temperature of the water is not given, so without much effect on the final result, we assume $T = 20°$ C, so that the kinematic viscosity is $\nu = 0.01 cm^2/s$, and $\rho = 1$ g/cm$^3$.

With this information, we estimate that at $Re = 2500$, $R(Re) = 2.5659 \times 10^4$, so that:

$$R(Re) = 0.0290 Re^{7/4}. \tag{S7}$$

This is serendipitously comparable to the largest external resistance used in our experiments (for $Re = 3000$, $R_{\rm Rotta}/R_{\rm large} \simeq 1$). Since we also observed intermittency, oscillations, and a non-negligible change in $Re$ ($\Delta Re$, see Fig. S3) for this external resistance, we surmise that if Rotta had done experiments for $Re \gtrsim 3000$, he also would have observed the same. Since the $Re \lesssim 3000$ regime is without growing slugs, which were an original ingredient in the proposed mechanism, we conclude that Rotta did not, in fact, properly test Prandtl and Tietjens' mechanism.

## V. ESTIMATE OF EXTERNAL RESISTANCE $R$ FROM BARKLEY ET AL. [1]

Here we estimate the resistance of the resistor in the experiments of Ref. [1]. To our knowledge, this experiment went further than any other in trying to maximize the external resistance to try and maintain a constant flow rate for a constant pressure drop flow. To estimate $R(Re)$, we use Eq. S7, where $\Delta P_{\rm tot} = \rho g h$, and we take a case where the flow is fully laminar. We also assume that like our external resistances, $R(Re) \propto Re^{7/4}$. Based on the information provided in the paper and methods section:

- $\Delta h = 2300$ cm.
- $D = 1$ cm.
- The pipe length is 1500 cm, and the perturbation is $200D$ downstream, so that $L = 1300$ cm.
- The temperature of the water is not given, so without much effect on the final result, we assume $T = 20°$ C, so that the kinematic viscosity is $\nu = 0.01 cm^2/s$, and $\rho = 1$ g/cm$^3$.

With this information, we estimate that at $Re = 3000$ (if we used $Re = 5000$ we would end up with a slightly lower estimate), $R(Re) = 5.3938 \times 10^5$, so that:

$$R(Re) = 0.4435 Re^{7/4}. \tag{S8}$$

Using this $R$ our predictions for the deviations in $Re$, $\Delta Re$ are in good agreement with their own observations ($\Delta Re/Re_0 \leq 0.5\%$). We used this estimate of $R(Re)$, which is much larger than any we achieved experimentally, with our model to estimate the span of intermittency as shown in Fig. 4 in the main text.

[1] D. Barkley, B. Song, V. Mukund, G. Lemoult, M. Avila, and B. Hof, Nature **526**, 550 (2015).
[2] J. Rotta, Ingenieur-Archiv **24**, 258 (1956).
[3] R. T. Cerbus, C.-C. Liu, G. Gioia, and P. Chakraborty, Physical Review Letters **120**, 054502 (2018).
[4] A. De Lozar and B. Hof, Philosophical Transactions of the Royal Society A: Mathematical, Physical and Engineering Sciences **367**, 589 (2009).
[5] M. Nishi, B. Ünsal, F. Durst, and G. Biswas, Journal of Fluid Mechanics **614**, 425 (2008).
